# Supplementary material for: Selecting and Pruning: A Differentiable Causal Sequentialized State-Space Model for Two-View Correspondence Learning
Source: arXiv:2503.17938 source file (2025-03-23)
Supplement: Supplementary file 1 [file _supplementary.tex]

%\input{_constants}
%\review % \review OR \cameraready
%
%\documentclass[10pt,twocolumn,letterpaper]{article}
%\input{cvpr_header}
%\myexternaldocument{_main}
%\begin{document}
%
%%% TITLE
%\title{\paperTitle}
%\author{\authorBlock}
%\maketitlesupplementary
%%%
%
%\appendix
%\input{12_appendix}
%
%{\small
%\bibliographystyle{ieeenat_fullname}
%\bibliography{11_references}
%}
%
%\end{document}
